# Supplementary material for: Blurring the boundaries between topological and non-topological phenomena in dots
Source: arXiv:1803.02936 ancillary file (2018-03-08)
Supplement: Supplementary file 1 [file Candido-SM.pdf]

Supplemental Material

# Blurring the boundaries between topological and non-topological phenomena in dots

Denis R. Candido,[1] M. E. Flatté,[2] and J. Carlos Egues[1,3]

[1]*Instituto de Física de São Carlos, Universidade de São Paulo, 13560-970, São Carlos, São Paulo, Brazil*

[2]*Department of Physics and Astronomy and Optical Science and Technology Center, University of Iowa, Iowa City, Iowa 52242, USA*

[3]*International Institute of Physics, Federal University of Rio Grande do Norte, 59078-970, P. O. Box 1613, Natal, Brazil*

(Dated: March 7, 2018)

## I. $InAs_{1-x}Bi_x$ QUANTUM WELLS: A NEW 2D TOPOLOGICAL INSULATOR.

The properties of III-V semiconductors doped with isoelectronic dopants that generate resonant states have been explored over the past fifteen years due to their dramatically smaller band gaps than the original host. The origin of the effect is the repulsion between the near-band-edge resonant state of the dopant and the band edge of the host. Dramatic changes in the band gap of GaAs through the addition of dilute nitrogen doping due to a resonant state in the conduction band, or through the addition of Bi due to a resonant state in the valence band, have been obtained. We use the experimentally obtained change in band gap of InAsBi of 58 meV/% Bi [1] for the electronic parameters of the bulk material. The resulting bulk material, sandwiched in a quantum well with symmetric AlSb barriers and grown on GaSb, is then studied using a superlattice electronic structure theory that has been applied to a broad range of narrow-gap semiconductor materials with inversion asymmetry and large spin-orbit interaction [2].

## II. EFFECTIVE BHZ PARAMETERS FOR $InAs_{0.85}Bi_{0.15}/AlSb$ QUANTUM WELLS.

The BHZ parameters $A$, $B$, $C$, $D$ and $M$ are obtained accordingly to Ref. [3] for our fourteen bulk band basis [2]. We calculate them for the a) topological trivial $InAs_{0.85}Bi_{0.15}$ QW with $d$ = 6 nm and b) topological non-trivial QW with $d$ = 8 nm. Their respective values of the BHZ parameters are given in Tab. I.

| $InAs_{1-x}Bi_x$ | d (nm) | A (meV.nm) | B (meV.nm$^2$) | C (meV) | D (meV.nm$^2$) | M (meV) |
|---|---|---|---|---|---|---|
| $x = 0.15$ | 6 | 543.2 | -201.7 | 0 | -180.0 | 16.1 |
| $x = 0.15$ | 8 | 488.0 | -339.3 | 0 | -300.0 | -15.5 |

Table I. Effective BHZ parameters for $InAs_{1-x}Bi_x$/AlSb QW with different well thickness (6 nm and 8 nm) and $x = 0.15$ of Bi concentration. For convenience we have chosen here $C = 0$ for all the cases.

## III. BHZ SOFT-WALL ENERGY LEVELS FOR A CYLINDRICAL QD.

Here we derive a generalization of the transcendental equation [Eq. (5) in the main text] for the BHZ Hamiltonian with a cylindrical soft-wall confinement having equal conduction and valence

barriers $M_O - M$ given by [4]

$$V_c = \begin{pmatrix} V(r)\,\sigma_z & 0 \\ 0 & V(r)\,\sigma_z \end{pmatrix}, \qquad V(r) = \begin{cases} 0 & r < R \\ M_O - M > 0 & r > R \end{cases} \tag{S1}$$

For the inner region ($r < R$) we have the regularized modified Bessel's functions at $r = 0$ (first kind)

$$\psi^{\pm,\,r<R}_{j_z,n}(r,\theta) = \sum_{\sigma=\pm} p^{\pm}_{j_z,n,\sigma} \begin{bmatrix} I_{j_z\mp\frac{1}{2}}(\lambda_\sigma r)\, e^{i\left(j_z\mp\frac{1}{2}\right)\theta} \\ \frac{D_+\lambda_\sigma^2 - E^{\pm}_{j_z,n} + C_+}{iA(\pm\lambda_\sigma)}\, I_{j_z\mp\frac{3}{2}}(\lambda_\sigma r)\, e^{i\left(j_z\mp\frac{3}{2}\right)\theta} \end{bmatrix} = \sum_{\sigma=\pm} p^{\pm}_{j_z,n,\sigma} \begin{bmatrix} I_{j_z\mp\frac{1}{2}}(\lambda_\sigma r)\, e^{i\left(j_z\mp\frac{1}{2}\right)\theta} \\ R^{\pm}_{j_z,n,\sigma}\, I_{j_z\mp\frac{3}{2}}(\lambda_\sigma r)\, e^{i\left(j_z\mp\frac{3}{2}\right)\theta} \end{bmatrix}, \tag{S2}$$

where $D_+ = D + B$, $C_+ = C + M$, $R^{\pm}_{j_z,n,\sigma} = \frac{\left(D_+\lambda_\sigma^2 - E^{\pm}_{j_z,n} + C_+\right)}{iA(\pm\lambda_\sigma)}$, and the other parameters have been defined in the main text (see definitions below Eq. (6)). For the outer region ($r > R$) we have the regularized modified Bessel's at $r \to \infty$ (second kind)

$$\psi^{\pm,r>R}_{j_z,n}(r,\theta) = \sum_{\sigma=\pm} r^{\pm}_{j_z,n,\sigma} \begin{bmatrix} K_{j_z\mp\frac{1}{2}}\left(\lambda^O_\sigma r\right) e^{i\left(j_z\mp\frac{1}{2}\right)\theta} \\ \frac{D_+\lambda^{O\,2}_\sigma - E^{\pm}_{j_z} + C_+}{-iA\left(\pm\lambda^O_\sigma\right)}\, K_{j_z\mp\frac{3}{2}}\left(\lambda^O_\sigma r\right) e^{i\left(j_z\mp\frac{3}{2}\right)\theta} \end{bmatrix} = \sum_{\sigma=\pm} r^{\pm}_{j_z,n,\sigma} \begin{bmatrix} K_{j_z\mp\frac{1}{2}}\left(\lambda^O_\sigma r\right) e^{i\left(j_z\mp\frac{1}{2}\right)\theta} \\ -R^{O,\pm}_{j_z,n,\sigma}\, K_{j_z\mp\frac{3}{2}}\left(\lambda^O_\sigma r\right) e^{i\left(j_z\mp\frac{3}{2}\right)\theta} \end{bmatrix}, \tag{S3}$$

with $\lambda^O_\sigma = \lambda_\sigma\left(M \to M^O\right)$ and $R^{O,\pm}_{j_z,n,\sigma} = R^{\pm}_{j_z,n,\sigma}\left(M \to M^O\right)$. To find the quantized energies of the system, we first need to match the continuity of the 1) wave function and 2) its derivative in the radial direction at $r = R$, yielding

$$\psi^{\pm,r<R}_{j_z,n}(r = R,\theta) = \psi^{\pm,r>R}_{j_z,n}(r = R,\theta), \tag{S4}$$

$$\partial_r\psi^{\pm,r<R}_{j_z,n}(r = R,\theta) = \partial_r\psi^{\pm,r>R}_{j_z,n}(r = R,\theta). \tag{S5}$$

Choosing $\theta = 0$, we combine Eqs. (S4) and (S5) in the following matrix equation

$$\begin{pmatrix} I_{j_z\mp\frac{1}{2}}(\lambda_+R) & I_{j_z\mp\frac{1}{2}}(\lambda_-R) & K_{j_z\mp\frac{1}{2}}\left(\lambda^O_+R\right) & K_{j_z\mp\frac{1}{2}}\left(\lambda^O_-R\right) \\ R^{\pm}_{j_z,n,+}I_{j_z\mp\frac{3}{2}}(\lambda_+R) & R^{\pm}_{j_z,n,-}I_{j_z\mp\frac{3}{2}}(\lambda_-R) & -R^{O,\pm}_{j_z,n,+}K_{j_z\mp\frac{3}{2}}\left(\lambda^O_+R\right) & -R^{O,\pm}_{j_z,n,-}K_{j_z\mp\frac{3}{2}}\left(\lambda^O_-R\right) \\ \partial_rI_{j_z\mp\frac{1}{2}}(\lambda_+R) & \partial_rI_{j_z\mp\frac{1}{2}}(\lambda_-R) & \partial_rK_{j_z\mp\frac{1}{2}}\left(\lambda^O_+R\right) & \partial_rK_{j_z\mp\frac{1}{2}}\left(\lambda^O_-R\right) \\ R^{\pm}_{j_z,n,+}\partial_rI_{j_z\mp\frac{3}{2}}(\lambda_+R) & R^{\pm}_{j_z,n,-}\partial_rI_{j_z\mp\frac{3}{2}}(\lambda_-R) & -R^{O,\pm}_{j_z,n,+}\partial_rI_{j_z\mp\frac{3}{2}}\left(\lambda^O_+R\right) & -R^{O,\pm}_{j_z,n,-}\partial_rK_{j_z\mp\frac{3}{2}}\left(\lambda^O_-R\right) \end{pmatrix} \begin{pmatrix} p^{\pm}_{j_z,n,+} \\ p^{\pm}_{j_z,n,-} \\ -r^{\pm}_{j_z,n,+} \\ -r^{\pm}_{j_z,n,-} \end{pmatrix} = 0, \tag{S6}$$

whose determinant when set to zero determines all the non-trivial quantized energy levels for the soft wall case. We solve Eq. (S6) for a soft wall barrier $M_O = 2$ eV using the same set of BHZ

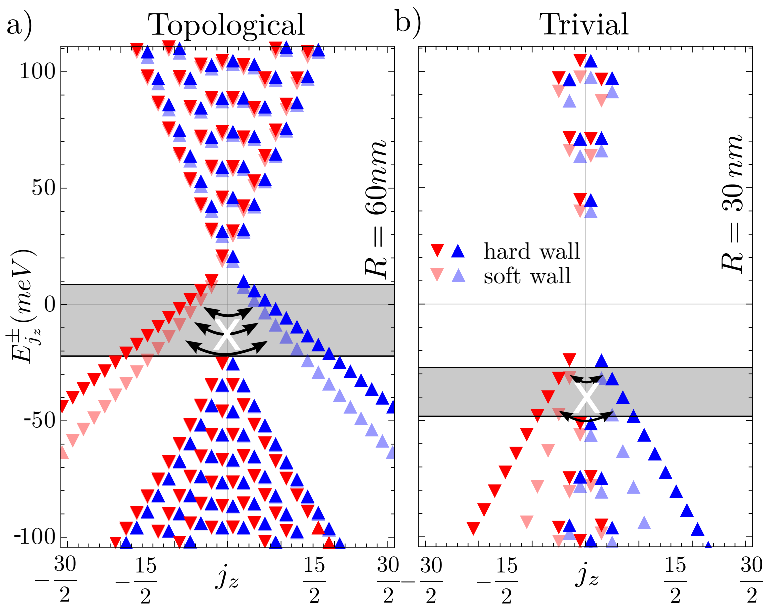


Figure S1. (a) Topological QD energy levels as a function of the total angular momentum $j_z$ for the soft ($M_O = 2$ eV) and hard wall ($M_O \to \infty$) cases for $R = 60$nm. (b) Same as (a) but for a trivial QD with $R = 30$nm. The arrows denote forbidden transitions between spin up and spin down states of the BHZ blocks, blue and red symbol, respectively.

parameters and QD radii as that of Fig. 1(c) and 1(e). We plot in Fig. (S1) both the soft and hard wall QD energy levels as a matter of comparison. The solid symbols represent the hard wall case, while the fading color symbols represent the soft wall case. We see that the bulk-like and the edge-like states of both the topological and trivial QDs behave similarly for soft wall confinement. The bulk-like levels are shifted by a small amount independent of $j_z$, while the edge states are shifted by a larger amount proportional to $j_z$. We emphasize that even in the presence of the soft wall confinement we still find protected trivial helical edge states within the energy range indicated by the gray area of Fig. S1(b).

We assume that $M_O = 2$ eV represents a realistic AlSb soft wall barrier heterostructure. Although this choice gives just two pairs of *geometrically protected* trivial helical edge states, the soft wall barrier (possibly) modulated by tunable gates on our QWs could lead to a full control of the number of protected trivial helical edge states.

## IV. ORDINARY InAs QD HAMILTONIAN.

In contrast to the topologically trivial and non-trivial InAsBi QWs, the ordinary InAs/AlSb QW with its large subband gap can be described approximately by decoupled parabolic dispersions using realistic effective masses. Thus we solve for the corresponding conduction and valence QD energy levels independently. The effective Hamiltonian for (the doubly-degenerate) lowest conduction $|C_1\pm\rangle$ (with energy $E_{C_1}$) and highest valence $|H_1\pm\rangle$ (with energy $E_{H_1}$) QW subbands reads

$$\mathcal{H}_{InAs} = \begin{bmatrix} \frac{\hbar^2}{2m_{C_1}}\boldsymbol{k}^2 + E_{C_1} & 0 & 0 & 0 \\ 0 & \frac{\hbar^2}{2m_{H_1}}\boldsymbol{k}^2 - E_{H_1} & 0 & 0 \\ 0 & 0 & \frac{\hbar^2}{2m_{C_1}}\boldsymbol{k}^2 + E_{C_1} & 0 \\ 0 & 0 & 0 & \frac{\hbar^2}{2m_{H_1}}\boldsymbol{k}^2 - E_{H_1} \end{bmatrix}. \tag{S7}$$

where realist $\boldsymbol{k.p}$ calculations [2] for the InAs/AlSb QW with thickness $d = 6$ nm yield effective masses $m_{C_1} = 0.0473\, m_0$ and $m_{H_1} = -0.2163\, m_0$ and $E_{C_1} - E_{H_1} = 401.4$ meV. The respective wave functions for cylindrical hard-wall confinement [Eq. (2) in the main text] can be straightforwardly obtained

$$\psi^{C_1\pm}_{j_z,n}(r,\theta) = p_{j_z,n} I_{j_z\mp\frac{1}{2}}(\lambda_{C_1} r)\, e^{i(j_z\mp\frac{1}{2})\theta}, \tag{S8}$$

$$\psi^{H_1\pm}_{j_z,n}(r,\theta) = q_{j_z,n} I_{j_z\mp\frac{3}{2}}(\lambda_{H_1} r)\, e^{i(j_z\mp\frac{3}{2})\theta}, \tag{S9}$$

with $\lambda_{C_1} = \sqrt{\frac{E^{C_1\pm}_{j_z,n} - E_{C_1}}{-\frac{\hbar^2}{2m_{C_1}}}}$, $\lambda_{HH_1} = \sqrt{\frac{E^{H_1\pm}_{j_z,n} + E_{H_1}}{-\frac{\hbar^2}{2m_{H_1}}}}$ and $p_{j_z,n}$, $q_{j_z,n}$ being the normalization factors. The energies are determined by imposing the vanishing of the above wave functions at $r = R$, yielding

$$E^{C_1\pm}_{j_z,n} = E_{C_1} + \frac{\hbar^2}{2m_{C_1}}\left(\frac{\alpha^n_{j_z\mp\frac{1}{2}}}{R}\right)^2, \tag{S10}$$

$$E^{H_1\pm}_{j_z,n} = -E_{H_1} + \frac{\hbar^2}{2m_{H_1}}\left(\frac{\alpha^n_{j_z\mp\frac{3}{2}}}{R}\right)^2, \tag{S11}$$

where $\alpha^n_{j_z\mp\frac{1}{2}}$ ($\alpha^n_{j_z\mp\frac{3}{2}}$) are the $n^{th}$-order zero of the modified Bessel's function of order $j_z \mp \frac{1}{2}$ ($j_z \mp \frac{3}{2}$). Using now that the modified Bessel's functions satisfy $I_{j_z\mp\frac{1}{2}}(\lambda r) = I_{-j_z\pm\frac{1}{2}}(\lambda r)$ and $I_{j_z\mp\frac{3}{2}}(\lambda r) =$

$I_{-j_z\pm\frac{3}{2}}(\lambda r)$, we find the following degeneracies

$$E^{C_1\pm}_{j_z\mp\frac{1}{2},n} = E^{C_1\pm}_{-j_z\pm\frac{1}{2},n}, \tag{S12}$$

$$E^{H_1\pm}_{j_z\mp\frac{3}{2},n} = E^{H_1\pm}_{-j_z\pm\frac{3}{2},n}. \tag{S13}$$

Together with the degeneracy due to TRS, we find for each $j_z$ level (with $j_z \neq \pm\frac{1}{2}$ for $C_1\pm$ and $j_z \neq \pm\frac{3}{2}$ for $H_1\pm$) the 4-fold degeneracies discussed in the main text

$$E^{C_1\pm}_{j_z\mp\frac{1}{2},n} = E^{C_1\mp}_{-(j_z\mp\frac{1}{2}),n} = E^{C_1\pm}_{-j_z\pm\frac{1}{2},n} = E^{C_1\mp}_{-(-j_z\pm\frac{1}{2}),n}, \tag{S14}$$

$$E^{H_1\pm}_{j_z\mp\frac{3}{2},n} = E^{H_1\mp}_{-(j_z\mp\frac{3}{2}),n} = E^{H_1\pm}_{-j_z\pm\frac{3}{2},n} = E^{H_1\mp}_{-(-j_z\pm\frac{3}{2}),n}. \tag{S15}$$

Additionally, the helical character in the ordinary InAs QD is also absent since the degenerate states Eqs. (S12) and (S13) have circulating currents with opposite propagation direction. The degenerate levels Eq.S12-S13 are not helical at all. Next we estimate the influence of the electron-hole mixing and the spin-orbit couplings of the Rashba and Dresselhaus types on the energy spectrum of ordinary InAs QDs. For completeness, in Sec. V we also assess the effect of the intrinsic bulk-inversion asymmetry (BIA) term on the Bi-based BHZ QD energy levels.

### A. Ordinary InAs QD in the presence of $C_1$-$H_1$ mixing

Here we investigate the influence of including the mixing between the $|C_1\pm\rangle$ and $|H_1\pm\rangle$ subbands in the effective InAs/AlSb QW Hamiltonian, Eq. (S7). We model this coupling through the $\pm A'k_\pm$ terms in the Hamiltonian

$$\mathcal{H}^{C_1-H_1}_{InAs} = \begin{bmatrix} \frac{\hbar^2}{2m_{C_1}}\boldsymbol{k}^2 + E_{C_1} & A'k_+ & 0 & 0 \\ A'k_- & \frac{\hbar^2}{2m_{H_1}}\boldsymbol{k}^2 - E_{H_1} & 0 & 0 \\ 0 & 0 & \frac{\hbar^2}{2m_{C_1}}\boldsymbol{k}^2 + E_{C_1} & -A'k_- \\ 0 & 0 & -A'k_+ & \frac{\hbar^2}{2m_{H_1}}\boldsymbol{k}^2 - E_{H_1} \end{bmatrix}. \tag{S16}$$

The new energies thus read

$$E_\pm = \frac{E_{C_1}+E_{H_1}}{2} + \frac{\hbar^2}{4}\left(\frac{1}{m_{C_1}} + \frac{1}{m_{H_1}}\right)\boldsymbol{k}^2 \pm \sqrt{\left[\frac{E_{C_1}-E_{H_1}}{2} + \frac{\hbar^2}{4}\left(\frac{1}{m_{C_1}} - \frac{1}{m_{H_1}}\right)\boldsymbol{k}^2\right]^2 + (A'\boldsymbol{k})^2}. \tag{S17}$$

To obtain an estimate for the QD energies, we now make $|\boldsymbol{k}| \approx \frac{1}{R}$ in the above formula (the QD radius is a reasonable assumption for $|\boldsymbol{k}|$) and use simple perturbative expansion to find

$$\Delta E^{mix}_{C_1-H_1} \approx \frac{\left(\frac{A}{R}\right)^2}{E_{C_1} - E_{H_1}}. \tag{S18}$$

Using $E_{C_1} - E_{H_1} = 401.4$ meV (Sec. IV), $A' \approx 300$ meV.nm (Tab. S1) and $R = 30$ nm, we obtain

$$\Delta E^{mix}_{C_1-H_1} \approx 1 \text{ meV}, \tag{S19}$$

which is small as compared to the QD energy level broadening due to, e.g., coupling to leads (see below Sec. IX C.)

### B. Ordinary InAs QD in the presence of spin orbit Rashba term

Although our calculations (main text) were done by considering symmetric InAs/AlSb QWs, we can estimate the shift in the QD energy levels due to spin-orbit interaction by including the linear Rashba term [6, 7] arising from a possible structural inversion asymmetry (SIA). For simplicity, we only consider the Rashba term in the electron subspace. In this case our Hamiltonian reads

$$\mathcal{H}^{Rashba}_{InAs} = \begin{bmatrix} \frac{\hbar^2}{2m_{C_1}}\boldsymbol{k}^2 + E_{C_1} & 0 & -i\alpha k_- & 0 \\ 0 & \frac{\hbar^2}{2m_{H_1}}\boldsymbol{k}^2 - E_{H_1} & 0 & 0 \\ i\alpha k_+ & 0 & \frac{\hbar^2}{2m_{C_1}}\boldsymbol{k}^2 + E_{C_1} & 0 \\ 0 & 0 & 0 & \frac{\hbar^2}{2m_{H_1}}\boldsymbol{k}^2 - E_{H_1} \end{bmatrix}. \tag{S20}$$

The new conduction energies are given by

$$E^{\pm}_{C_1,SIA} = E_{C_1} + \frac{\hbar^2\boldsymbol{k}^2}{2m_{C_1}} \pm \alpha\,|\boldsymbol{k}|\,. \tag{S21}$$

Using the realistic $\alpha = 28$ meV.nm [5] and again making $|\boldsymbol{k}| \approx \frac{1}{R}$ with $R = 30$ nm, we obtain the QD energy level shift due the Rashba spin orbit coupling

$$\Delta E_{C_1,SIA} \approx \pm\frac{\alpha}{R} \rightarrow \Delta E_{C_1,R} \approx 0.9 \text{ meV}, \tag{S22}$$

which is also small [c.f., Eq. (S19)].

### C. Ordinary InAs QD in the presence of bulk inversion asymmetry term (BIA)

Now we take into account the influence of the intrinsic bulk inversion asymmetry (BIA) term [7], which arises from the lack of inversion symmetry in the Zincblende structure. Here consider only the BIA term within the electron subspace Using the leading order BIA terms [8, 9] in Eq. (S7) we obtain

$$\mathcal{H}_{InAs}^{BIA} = \begin{bmatrix} \frac{\hbar^2}{2m_{C_1}}\boldsymbol{k}^2 + E_{C_1} & 0 & -\beta k_+ & 0 \\ 0 & \frac{\hbar^2}{2m_{H_1}}\boldsymbol{k}^2 - E_{H_1} & 0 & 0 \\ -\beta k_- & 0 & \frac{\hbar^2}{2m_{C_1}}\boldsymbol{k}^2 + E_{C_1} & 0 \\ 0 & 0 & 0 & \frac{\hbar^2}{2m_{H_1}}\boldsymbol{k}^2 - E_{H_1} \end{bmatrix}, \tag{S23}$$

which has eigenvalues

$$E_{C_1,BIA}^{\pm} = E_{C_1} + \frac{\hbar^2\boldsymbol{k}^2}{2m_{C_1}} \pm \beta\,|\boldsymbol{k}|\,. \tag{S24}$$

The linear Dresselhaus parameter for InAs/AlSb QW is typically $\beta \approx 5$ meV.nm [5]. Using then $|\boldsymbol{k}| \approx \frac{1}{R}$ with $R = 30$ nm, we obtain the following shift in the QD energy levels

$$\Delta E_{C_1,BIA} \approx \frac{\beta}{R} \rightarrow \Delta E_{C_1} \approx 0.17 \text{ meV}, \tag{S25}$$

which is also negligible.

## V. TRIVIAL $InAs_{0.85}Bi_{0.15}$ QD IN THE PRESENCE OF BIA

In our trivial $InAs_{0.85}Bi_{0.15}$ QD case, the presence of the BIA terms should be more important as compared to the previous case (ordinary InAs QD). The reason lies in the fact that the Bi-based compounds have larger spin-orbit interaction thus possibly enhancing the strength of the

BIA terms. In leading order, the BHZ Hamiltonian with BIA reads [11]

$$\mathcal{H}_{InAsBi}^{BIA} = C - D\boldsymbol{k}^2 + \begin{bmatrix} M - B\boldsymbol{k}^2 & Ak_+ & 0 & -\Delta_{BIA} \\ Ak_- & -M + B\boldsymbol{k}^2 & \Delta_{BIA} & 0 \\ 0 & \Delta_{BIA} & M - B\boldsymbol{k}^2 & -Ak_- \\ -\Delta_{BIA} & 0 & -Ak_+ & -M + B\boldsymbol{k}^2 \end{bmatrix}, \tag{S26}$$

with eigenenergies given by [4]

$$E_{BHZ}^{\pm,s=\pm}(\boldsymbol{k}, \Delta_{BIA}) = C - D\boldsymbol{k}^2 \pm \sqrt{(A\,|\boldsymbol{k}| + s\Delta)^2 + \left(M - B\boldsymbol{k}^2\right)^2}. \tag{S27}$$

Using the parameters on Tab. S1, assuming $|\boldsymbol{k}| \approx \frac{1}{R}$ with $R = 30$ nm, and $\Delta_{BIA} = 4$ meV (twice the value of HgTe/CdTe [11]) we estimate the shift in valence energy due to the $\Delta_{BIA}$ as

$$E_{BHZ}^{-,s=\pm}\left(\frac{1}{R}, \Delta_{BIA}\right) - E_{BHZ}^{-,s=\pm}\left(\frac{1}{R}, \Delta_{BIA} = 0\right) \approx 2\text{meV}. \tag{S28}$$

This energy shift is comparable to the energy level broadening due to the coupling to the leads (see Sec. IX C.).

## VI. PERSISTENCE OF THE GEOMETRICALLY PROTECTED TRIVIAL HELICAL EDGE STATES FOR INCREASING QD RADII.

We investigate here the persistence of the protected trivial helical edge-like states as a function of the QD radius $R$. Due to the distinct wave function character between the edge-like and bulk-like states, their energies behave differently as a function of QD radius $R$. For the trivial edge-like states, the wave functions are more localized at the interface ($r = R$) with the corresponding eigenenergies not so sensitive to the QD size $R$. On the other hand, the bulk-like wave functions are extended through the whole QD and have very sensitive eigenenergies to R changes. Due to this different sensitivity to the QD radius, the energies of the edge-like and bulk-like states can cross each other as we increase $R$, thus destroying the robustness of the trivial edge-like states against scattering. We plot in Fig. (S2) the energy levels as a function of $R$ for the four spin up trivial helical edge-like energies $j_z = \frac{3}{2}, \frac{5}{2}, \frac{7}{2}, \frac{9}{2}$ in the gray area of Fig. 1(e) together with the nearest bulk-like energy level $j_z = \frac{1}{2}$ outside the gray area. The bulk-like energy level is more sensitive to the

QD radius and cross the edge-like energy levels at $R_{c1} = 44$ nm and $R_{c2} = 106$ nm (see red points in Fig. (S2)), where the number of *geometrically protected* trivial helical edge states is decreased by one at each crossing. Although the number of *geometrically protected* trivial helical states have decreased, the four trivial helical edge states persist for a wide radius range $0 < R < 44$nm. We emphasize that even for $R > 44$ nm, where we have just three pairs of protected trivial helical edge-like states, our main feature will still remain for a reasonable energy window. As for the

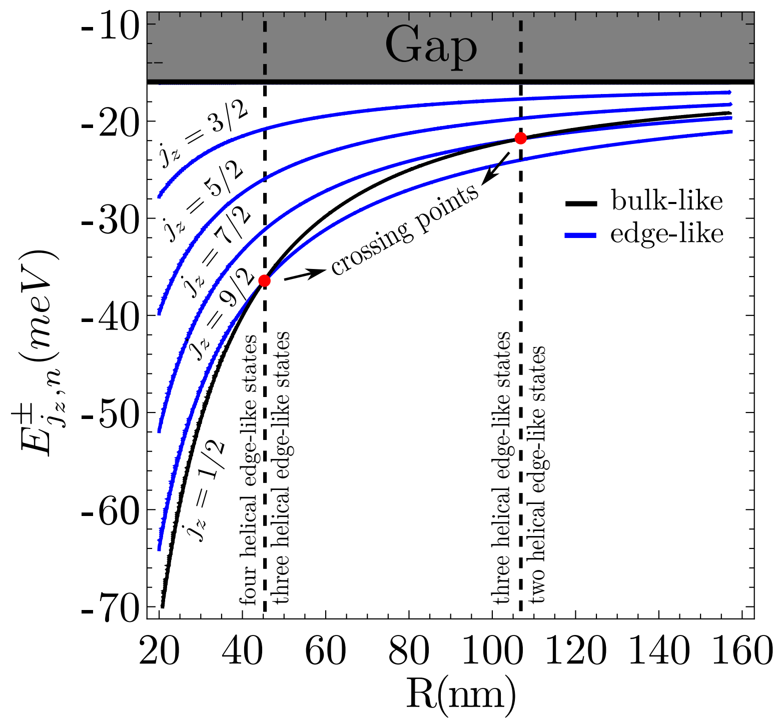


Figure S2. (Color online) Trivial spin up edge-like energy levels $j_z = \frac{3}{2}, \frac{5}{2}, \frac{7}{2}, \frac{9}{2}$ within the gray area of Fig. 1e) (main text) and their nearest bulk-like energy level $j_z = \frac{1}{2}$ plotted as function of the QD radius. The red dots indicate the crossing points where the number of the protected trivial edge states decreases by one.

topological QDs, we find that their bulk-like and edge-like states behave similar to the to the ones of the trivial QDs. Thus we still have the similar energy crossing between bulk and edge states arising from their different sensitivity to the QD radius.

## VII. EXTENDED QD ENERGY LEVELS FOR DIFFERENT BHZ PARAMETER SETS

We plot in Fig. (S3) the QD energy levels for three different sets of HgTe/CdTe BHZ parameters given in Refs. [4, 10, 11]. Surprisingly, the existence of trivial helical edge states protected against elastic scattering holds, showing thus this is not a particular feature of our $InAs_{0.85}Bi_{0.15}$ QD. On

the other hand, the number of protected trivial helical edge states within the gray area depends strongly on the BHZ parameters. We find that the smaller the difference $|D| - |B|$ with $D < 0$ ($D > 0$) is the larger the number of protected helical edge states in the valence (conduction) subspace are, thus enhancing the possibility of being experimentally controllable.

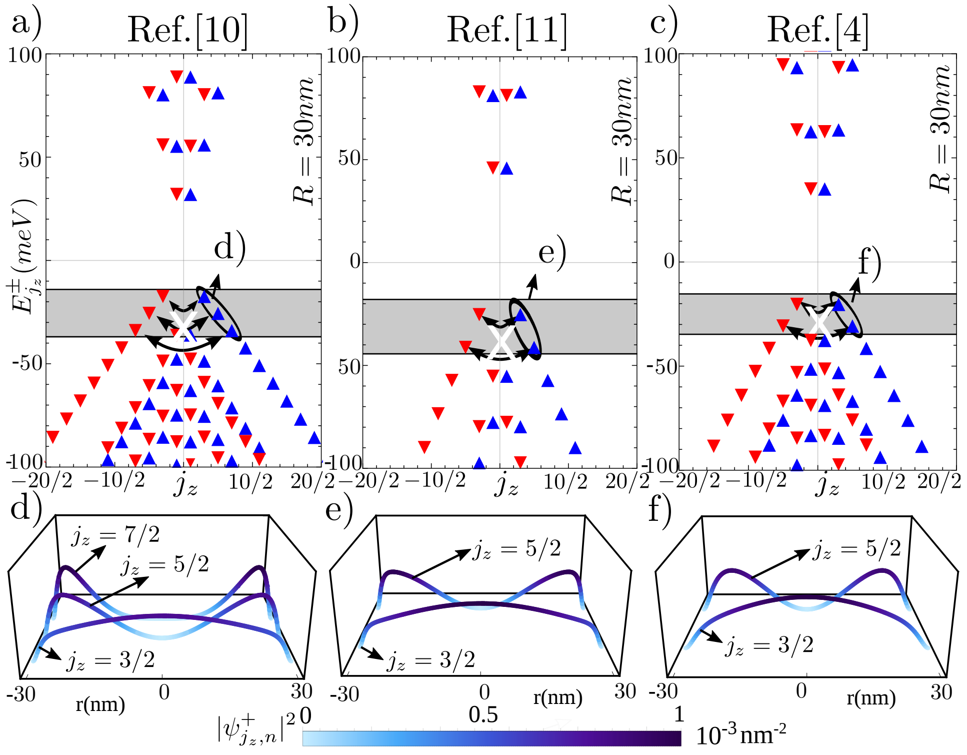


Figure S3. (Color online) a) Even (circle) and odd (triangle) QD energy levels as a function of the total angular momentum $j_z$ for the BHZ parameters of Ref. [10] with $R = 30$ nm; b) Same as a) for parameters from Ref. [11]. c) Same as a) for parameters from Ref. [4]. The arrows denote the forbidden transitions between spin up and spin down states of the BHZ blocks, blue and red symbol, respectively. d), e) and f): Modulus square of the spin up wave functions $|\Psi|^2$ for the edge grouped by the ellipses in a), b) and c)

## VIII. CIRCULATING CURRENT DENSITY

In this section we derive in details the circulating current formula Eq. (7). For practical reasons, we write the total wave function Eq. (6) as

$$\psi^{\pm}_{j_z,n}\left(r,\theta,E^{\pm}_{j_z,n}\right) = \frac{N}{\sqrt{2\pi}}\left[I^{j_z\mp\frac{1}{2},n}_{E_1}(r)\, e^{i\left(j_z\mp\frac{1}{2}\right)\theta} \quad \pm i\, I^{j_z\mp\frac{3}{2},n}_{HH_1}(r)\, e^{i\left(j_z\mp\frac{3}{2}\right)\theta}\right]^T, \qquad \text{(S29)}$$

with

$$I_{E_1}^{j_z\mp\frac{1}{2},n}\left(r\right)=I_{j_z\mp\frac{1}{2}}\left(\lambda_+\left(E_{j_z,n}^{\pm}\right)r\right)-\frac{I_{j_z\mp\frac{1}{2}}\left(\lambda_+\left(E_{j_z,n}^{\pm}\right)R\right)}{I_{j_z\mp\frac{1}{2}}\left(\lambda_-\left(E_{j_z,n}^{\pm}\right)R\right)}I_{j_z\mp\frac{1}{2}}\left(\lambda_-\left(E_{j_z,n}^{\pm}\right)r\right), \tag{S30}$$

$$I_{HH_1}^{j_z\mp\frac{3}{2},n}\left(r\right)=\frac{D_+\lambda_+^2\left(E_{j_z,n}^{\pm}\right)-E_{j_z,n}^{\pm}+C_+}{\pm iA\lambda_+\left(E_{j_z,n}^{\pm}\right)}\left(I_{j_z\mp\frac{3}{2}}\left(\lambda_+\left(E_{j_z,n}^{\pm}\right)r\right)-\frac{I_{j_z\mp\frac{3}{2}}\left(\lambda_+\left(E_{j_z,n}^{\pm}\right)R\right)}{I_{j_z\mp\frac{3}{2}}\left(\lambda_-\left(E_{j_z,n}^{\pm}\right)R\right)}I_{j_z\mp\frac{3}{2}}\left(\lambda_-\left(E_{j_z,n}^{\pm}\right)r\right)\right), \tag{S31}$$

and $N$ being the normalization factor. The wave function in Eq.(S29) is obtained within the BHZ model in the usual basis $|E_1+\rangle, |HH_1+\rangle, |E_1-\rangle$ and $|HH_1-\rangle$ defined by [3]

$$|E_1\pm\rangle=f_1^{\pm}\left(z\right)\left|\Gamma_6\pm\frac{1}{2}\right\rangle+f_4^{\pm}\left(z\right)\left|\Gamma_8\pm\frac{1}{2}\right\rangle, \tag{S32}$$

$$|HH_1\pm\rangle=f_3^{\pm}\left(z\right)\left|\Gamma_8\pm\frac{3}{2}\right\rangle, \tag{S33}$$

where $f_i^{\pm}(z)$ are the QW envelope functions and $|\Gamma_i\pm\rangle$ are the periodic part of Bloch functions at $\Gamma$ point $\left|u_{i=1,2,3,4,5,6}\right\rangle = \left\{\left|\Gamma_6,\frac{1}{2}\right\rangle,\left|\Gamma_6,-\frac{1}{2}\right\rangle,\left|\Gamma_8,\frac{3}{2}\right\rangle,\left|\Gamma_8,\frac{1}{2}\right\rangle,\left|\Gamma_8,-\frac{1}{2}\right\rangle,\left|\Gamma_8,-\frac{3}{2}\right\rangle\right\}$ [3]. Using now Eqs. (S29)-(S33), we write the total wave function as

$$\psi_{j_z,n}^{\pm}=\frac{N}{\sqrt{2\pi}}\left[I_{E_1}^{j_z\mp\frac{1}{2},n}\left(r\right)e^{i\left(j_z\mp\frac{1}{2}\right)\theta}\left(f_1^{\pm}\left(z\right)\left|\Gamma_6,\pm\frac{1}{2}\right\rangle+f_4^{\pm}\left(z\right)\left|\Gamma_8,\pm\frac{1}{2}\right\rangle\right)\pm i\,I_{HH_1}^{j_z\mp\frac{3}{2},n}\left(r\right)e^{i\left(j_z\mp\frac{3}{2}\right)\theta}f_3^{\pm}\left(z\right)\left|\Gamma_8,\pm\frac{3}{2}\right\rangle\right], \tag{S34}$$

Since now we have our wave function written as a product of envelope functions and the periodic parts of the Bloch functions at $\Gamma$ point, $\psi_{j_z,n}^{\pm}\left(\boldsymbol{r}\right)=\sum_i F_{i,j_z,n}^{\pm}\left(r,\theta,z\right)u_i\left(\boldsymbol{r}\right)$, we use the formula of the average (over the unit cell) current density [12, 13],

$$\left\langle \boldsymbol{j}_{j_z,n}^{\pm}\right\rangle\left(\boldsymbol{r}\right)=\frac{e\hbar}{m_0}Im\sum_{i,j}\left\{F_{i,j_z,n}^{*}\left(\boldsymbol{r}\right)F_{j,j_z,n}\left(\boldsymbol{r}\right)\langle u_i|\boldsymbol{\nabla}\left|u_j\right\rangle+\delta_{ij}F_{i,j_z,n}^{*}\left(\boldsymbol{r}\right)\boldsymbol{\nabla}F_{j,j_z,n}\left(\boldsymbol{r}\right)\right\}, \tag{S35}$$

to obtain the final formula for our problem,

$$\left\langle \boldsymbol{j}_{j_z,n}^{\pm}\right\rangle\left(\boldsymbol{r}\right)=\left\langle \boldsymbol{j}_{j_z,n}^{\pm}\right\rangle_b\left(\boldsymbol{r}\right)+\left\langle \boldsymbol{j}_{j_z,n}^{\pm}\right\rangle_e\left(\boldsymbol{r}\right), \tag{S36}$$

where

$$\left\langle \boldsymbol{j}_{j_z,n}^{\pm}\right\rangle_b=\pm eN^2\frac{\sqrt{2}P}{2\pi\hbar}\left|f_1^{\pm}\left(z\right)\right|\left|f_3^{\pm}\left(z\right)\right|I_{E_1}^{j_z\mp\frac{1}{2},n}\left(r\right)I_{HH_1}^{j_z\mp\frac{3}{2},n}\left(r\right)\hat{\theta}, \tag{S37}$$

and

$$\left\langle \boldsymbol{j}^{\pm}_{j_z,n} \right\rangle_e = \frac{\hbar e N^2}{2\pi r\, m_0} \left\{ \left( j_z \mp \frac{1}{2} \right) \left[ \left| f_1^{\pm}(z) \right|^2 + \left| f_4^{\pm}(z) \right|^2 \right] \left| I_{E_1}^{j_z \mp \frac{1}{2},n}(r) \right|^2 + \left( j_z \mp \frac{3}{2} \right) \left| f_3^{\pm}(z) \right|^2 \left| I_{HH_1}^{j_z \mp \frac{3}{2},n}(r) \right|^2 \right\} \hat{\theta}. \tag{S38}$$

We emphasize that $\boldsymbol{r}$ here denotes the center of the unit cell position (see Ref. [12, 13] for details). The first term $\left\langle \boldsymbol{j}^{\pm}_{j_z,n} \right\rangle_b$ is the "Bloch velocity" contribution to the average current as it stems from the periodic Bloch functions, while the second term $\left\langle \boldsymbol{j}^{\pm}_{j_z,n} \right\rangle_e$ is the contribution from the envelope functions. From Eq. (S30) and (S31) we note that $I_{E_1}^{j_z \mp \frac{1}{2},n}(r) = I_{E_1}^{-j_z \pm \frac{1}{2},n}(r)$ and $I_{HH_1}^{j_z \mp \frac{3}{2},n}(r) = I_{HH_1}^{-j_z \pm \frac{3}{2},n}(r)$, yielding

$$\left\langle \boldsymbol{j}^{\pm}_{j_z,n} \right\rangle (\boldsymbol{r}) = - \left\langle \boldsymbol{j}^{\mp}_{-j_z,n} \right\rangle (\boldsymbol{r}), \tag{S39}$$

which corresponds to the helical property of the QD levels, i.e., states with opposite $j_z$ and spin (±) propagate in opposite angular direction.

### A. Envelope contribution to the circulating current

We plot in Fig. S4 the envelope function contribution $\left\langle \boldsymbol{j}^{\pm}_{j_z,n} \right\rangle_e$ to the circulating current for the spin up conduction levels of Fig. 2 (main text). All the density plots in Fig. S4 were multiplied by a factor of 50 in order to compare them to the total circulating current density plotted in Fig. 2. The magnitude of the color bar here is the same as in Fig. 2. In accordance with Refs. [12, 13] here we obtain a small envelope current contribution. Interestingly, the envelope current contribution for $j_z = 3/2$ is negligible and cannot be visualized using the amplification of 50 times. This stems from the fact that 1) the spin-up $j_z = 3/2$ states are almost purely $HH_1+$ states, so the $HH_1$ wave function components, $I_{HH_1}^{j_z - \frac{3}{2},n}$, are larger than the $E_1+$ ones, $I_{E_1}^{j_z - \frac{1}{2},n}$, and 2) for spin up $j_z = 3/2$ we have no envelope contribution from the $HH_1+$ subspace corresponding to the zero envelope orbital angular momentum $j_z - 3/2 = 0$. Using thus Eq. (S38) with 1) and 2) we find a negligible envelope circulating current.

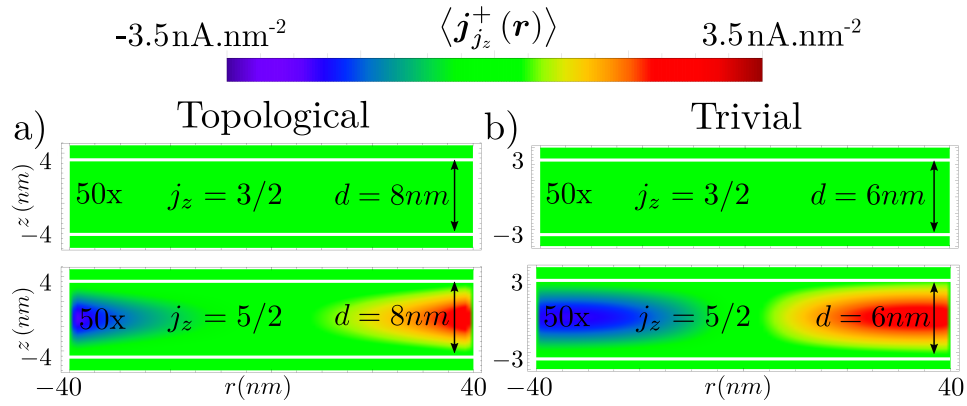


Figure S4. (Color online) (a) Spin-up envelope circulating current Eq. (S38) for the topological helical edge states $j_z = \frac{3}{2}$ and $j_z = \frac{5}{2}$ within the gray area of Fig. 1(c). (b) Spin-up circulating current for the trivial helical edge states $j_z = \frac{3}{2}$ and $j_z = \frac{5}{2}$ within the gray area of Fig. 1(e). The solid white lines correspond to the soft-wall QW barriers.

## IX. CONDUCTANCE CALCULATION

### A. Conductance formula

We derive here the conductance within the linear regime through non-interacting QD levels coupled to left (L) and right (R) leads [14–17]. As already discussed in the main text, for the conductance calculations we considerer two Kramers pairs, denoted by $|1\rangle = |j_{z1}, \uparrow\rangle$, $|2\rangle = |-j_{z1}, \downarrow\rangle$, $|3\rangle = |j_{z2}, \uparrow\rangle$ and $|4\rangle = |-j_{z2}, \downarrow\rangle$ with $\varepsilon_1 = \varepsilon_2$, $\varepsilon_3 = \varepsilon_4$, and $\varepsilon_i = \varepsilon_i(R, V_g)$. Although we have done the conductance calculation for the full Hamiltonian Eq. (9) of the main text (this result will be presented elsewhere), here we derive the conductance formula neglecting spin-flip processes as it is simpler analytically. The starting point is thus given by Eq. (9), which in the absence of spin-flip processes, i.e., $t_{14} = t_{23} = V^{2(4)}_{\boldsymbol{k}_\alpha\uparrow} = V^{1(3)}_{\boldsymbol{k}_\alpha\downarrow} = 0$ yields the following spin block diagonal Hamiltonian

$$H = \overbrace{\varepsilon_1 d_1^\dagger d_1 + \varepsilon_3 d_3^\dagger d_3 + \sum_{\boldsymbol{k}_\alpha\uparrow,\alpha} \varepsilon_{\boldsymbol{k}_\alpha\uparrow} c^\dagger_{\boldsymbol{k}_\alpha\uparrow} c_{\boldsymbol{k}_\alpha\uparrow} + \sum_{\boldsymbol{k}_\alpha\uparrow,\alpha}\left(V^1_{\boldsymbol{k}_\alpha\uparrow} d_1^\dagger c_{\boldsymbol{k}_\alpha\uparrow} + V^3_{\boldsymbol{k}_\alpha\uparrow} d_3^\dagger c_{\boldsymbol{k}_\alpha\uparrow}\right) + t_{13} d_1^\dagger d_3 + h.c.}^{=H_\uparrow} \tag{S40}$$

$$+ \overbrace{\varepsilon_2 d_2^\dagger d_2 + \varepsilon_4 d_4^\dagger d_4 + \sum_{\boldsymbol{k}_\alpha\downarrow,\alpha} \varepsilon_{\boldsymbol{k}_\alpha\downarrow} c^\dagger_{\boldsymbol{k}_\alpha\downarrow} c_{\boldsymbol{k}_\alpha\downarrow} + \sum_{\boldsymbol{k}_\alpha\downarrow,\alpha}\left(V^2_{\boldsymbol{k}_\alpha\downarrow} d_2^\dagger c_{\boldsymbol{k}_\alpha\downarrow} + V^4_{\boldsymbol{k}_\alpha\downarrow} d_4^\dagger c_{\boldsymbol{k}_\alpha\downarrow}\right) + t_{24} d_2^\dagger d_4 + h.c.}^{=H_\uparrow}, \tag{S41}$$

where the spin up Hamiltonian is represented schematically in Fig. S5. Because we are neglecting spin flip processes, we can calculate the conductance formula for just one particular spin component and multiply it by a factor of two in order to account for both spin components.

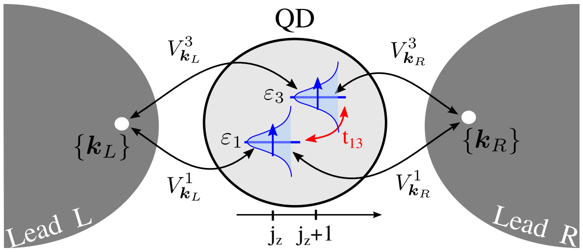


Figure S5. Schematic for the spin up QD Hamiltonian with levels $\varepsilon_1, \varepsilon_2$ coupled to each other through $t_{13}$ and coupled to left and right leads through $V^{1,3}_{\boldsymbol{k}_L\uparrow}$ and $V^{1,3}_{\boldsymbol{k}_R\uparrow}$.

The equations of motion for the retarded spin up Green functions yield

$$\begin{pmatrix} E-\varepsilon_1+i\eta-\sum_\alpha^{11} & 0 & 0 & -\sum_\alpha^{12}-t_{13}^* \\ 0 & E-\varepsilon_3+i\eta-\sum_\alpha^{33} & -\sum_\alpha^{31}-t_{13} & 0 \\ 0 & -\sum_\alpha^{13}-t_{13}^* & E-\varepsilon_1+i\eta-\sum_\alpha^{11} & 0 \\ -\sum_\alpha^{31}-t_{13} & 0 & 0 & E-\varepsilon_3+i\eta-\sum_\alpha^{33} \end{pmatrix} \begin{pmatrix} G_{11}^r(E) \\ G_{33}^r(E) \\ G_{13}^r(E) \\ G_{31}^r(E) \end{pmatrix} = \begin{pmatrix} 1 \\ 1 \\ 0 \\ 0 \end{pmatrix}, \tag{S42}$$

with $\sum_\alpha^{l,m} = \sum_{\boldsymbol{k}_\alpha,\alpha} \frac{V^l_{\boldsymbol{k}_\alpha\uparrow} V^{m*}_{\boldsymbol{k}_\alpha\uparrow}}{E-\varepsilon_{\boldsymbol{k}_\alpha\uparrow}+i\eta}$, $\alpha = L, R$ and $l, m = 1, 3$. Using the Meir-Wingreen [14] results assuming 1) equal left and right density of the states in the leads ($\rho_L = \rho_R$) and 2) equal spin-conserving coupling of the QD to left and right leads $\left(V^l_{\boldsymbol{k}_L\uparrow} = V^l_{\boldsymbol{k}_R\uparrow}\right)$. We find that the spin up current in the equilibrium regime reads

$$J_\uparrow = -\frac{e}{h}\int dE\,[f_L(E) - f_R(E)]\, Im\left[tr\left\{\boldsymbol{\Gamma}^{L(R)}\boldsymbol{G}^r\right\}\right], \tag{S43}$$

where $f_{L(R)}(E)$ is the Fermi-Dirac distribution of left (right) lead defined here as

$$f_L(E) = \frac{1}{\left(1+e^{\frac{E-\mu_L}{k_BT}}\right)}, \qquad f_R(E) = \frac{1}{\left(1+e^{\frac{E-\mu_R}{k_BT}}\right)}, \tag{S44}$$

where $k_B$ is the Boltzmann constant, $T$ is the temperature and $\mu_{L(R)}$ is the chemical potential of the left (right) lead. As for $\boldsymbol{\Gamma}^{L(R)}$ and $\boldsymbol{G}^r$, we have $\left(\boldsymbol{\Gamma}^{L(R)}\right)_{lm} = \Gamma^{L(R)}_{lm} = 2\pi\rho_{L(R)} V^l_{\boldsymbol{k}_{L(R)}\uparrow} V^{m*}_{\boldsymbol{k}_{L(R)}\uparrow}$ and $(\boldsymbol{G}^r)_{lm} = G^r_{lm}$, or explicitly,

$$\boldsymbol{\Gamma}^L = 2\pi\rho_L \begin{pmatrix} V^1_{\boldsymbol{k}_L\uparrow}V^{1*}_{\boldsymbol{k}_L\uparrow} & V^1_{\boldsymbol{k}_L\uparrow}V^{3*}_{\boldsymbol{k}_L\uparrow} \\ V^3_{\boldsymbol{k}_L\uparrow}V^{1*}_{\boldsymbol{k}_L\uparrow} & V^3_{\boldsymbol{k}_L\uparrow}V^{3*}_{\boldsymbol{k}_L\uparrow} \end{pmatrix}, \qquad \boldsymbol{G}^r = \begin{pmatrix} G^r_{11}(E) & G^r_{13}(E) \\ G^r_{31}(E) & G^r_{33}(E) \end{pmatrix}. \tag{S45}$$

Within linear response, i.e., $\mu_L - \mu_R = -eV$ with $eV \ll \mu_{L,R}$, we write

$$f_L(E) - f_R(E) \approx (\mu_L - \mu_R)\left(-\frac{\partial f_0}{\partial E}\right)_{E=\varepsilon_F} = (-eV)\left(-\frac{\partial f_0}{\partial E}\right)_{E=\varepsilon_F}, \tag{S46}$$

where $f_0$ is the equilibrium Fermi function $f_0(E) = 1/(e^{\frac{E-\varepsilon_F}{k_B T}} + 1)$ where we have taken the chemical potential as its $T = 0$ value, i.e., the Fermi energy $\mu = \varepsilon_F$. From Eq. (S43) the spin up conductance within linear response thus reads

$$\mathcal{G}_\uparrow = \left.\frac{dJ_\uparrow}{dV}\right|_{V=0} = \frac{e^2}{h}\int dE\, Im\left[tr\left\{\mathbf{\Gamma}^{L(R)}\boldsymbol{G}^r\right\}\right]\left.\left(-\frac{\partial f_0}{\partial E}\right)\right|_{E=\varepsilon_F}. \tag{S47}$$

Now we assume $k$-ndependent QD-lead couplings $V^l_{\boldsymbol{k}_L\uparrow} = V^l_L$, together with the wide band limit [18] where the constant 2D density of states in the leads $\rho_{L(,R)}$ is assumed to have a energy range much larger than the characteristic energies of our system, i.e., $\Delta\varepsilon_{L,R} \gg E$. We also assume the dependence of the QD energy levels on the gate $V_g$ as $\varepsilon_i(R, V_g) = \varepsilon_i(R) - eV_g$. Thus, the spin up conductance Eq. (S47) at $T = 0$ K reads

$$\mathcal{G}_\uparrow = \frac{e^2}{h}\frac{\left[\Gamma^L_3\left(\varepsilon_F - \varepsilon_1 + eV_g\right) + \Gamma^L_1\left(\varepsilon_F - \varepsilon_3 + eV_g\right) + 2t\Gamma^L_{13}\right]^2}{\left[\left(\varepsilon_F - \varepsilon_1 + eV_g\right)\left(\varepsilon_F - \varepsilon_3 + eV_g\right) - t^2\right]^2 + \left[\Gamma^L_3\left(\varepsilon_F - \varepsilon_1 + eV_g\right) + \Gamma^L_1\left(\varepsilon_F - \varepsilon_3 + eV_g\right) + 2t\Gamma^L_{13}\right]^2}, \tag{S48}$$

which exhibits $\frac{e^2}{h}$ conductance peaks centered at $\varepsilon_\pm$, corresponding to the poles of the $G_{11}$ and $G_{33}$ Green functions and determined by $(E - \varepsilon_1)(E - \varepsilon_3) - t^2 = 0$, i.e., $\varepsilon_\pm = \frac{\varepsilon_1+\varepsilon_3 \pm \sqrt{(\varepsilon_1-\varepsilon_3)^2+4t^2}}{2}$. We emphasize that the conductance formulas Eqs. (S33) and (S34) here correspond to a purely spin up conductance. Hence the total conductance follows

$$\mathcal{G} = \mathcal{G}_\uparrow + \mathcal{G}_\downarrow = 2\mathcal{G}_\uparrow. \tag{S49}$$

The total QD conductance $\mathcal{G}$ Eq. (S49) can also be written as

$$\mathcal{G} = \frac{2e^2}{h}\left\{\pi\Gamma^L_{11}\rho_1(\varepsilon_F) + \pi\Gamma^L_{22}\rho_2(\varepsilon_F)\right\} - \frac{4e^2}{h}\Gamma^L_{12} Im\left[G^r_{12}(\varepsilon_F)\right] \tag{S50}$$

where the first two terms (always positive definite) correspond to the conductance via the two QD levels and the last one represents the interference term [15–17].

### B. Diagonal QD level operators

The QD Hamiltonian sketched in Fig. S5 in the absence of coupling to the leads is given by

$$H_{QD} = \begin{pmatrix} d_1^\dagger & d_3^\dagger \end{pmatrix} \begin{pmatrix} \varepsilon_1 & t \\ t & \varepsilon_3 \end{pmatrix} \begin{pmatrix} d_1 \\ d_3 \end{pmatrix}, \tag{S51}$$

and has the following diagonal form

$$H = \begin{pmatrix} d_+^\dagger & d_-^\dagger \end{pmatrix} \begin{pmatrix} \varepsilon_+ & 0 \\ 0 & \varepsilon_- \end{pmatrix} \begin{pmatrix} d_+ \\ d_- \end{pmatrix}. \tag{S52}$$

with

$$d_+^\dagger = \frac{t\, d_1^\dagger + (\varepsilon_+ - \varepsilon_1)\, d_2^\dagger}{\sqrt{t^2 + (\varepsilon_+ - \varepsilon_1)^2}}, \qquad d_-^\dagger = \frac{t\, d_1^\dagger + (\varepsilon_- - \varepsilon_1)\, d_2^\dagger}{\sqrt{t^2 + (\varepsilon_- - \varepsilon_1)^2}}. \tag{S53}$$

We rewrite now the Hamiltonian that couples the QD to the leads using the diagonal $d_+, d_-$ operators, yielding

$$H_{Lead-QD} = \sum_{\boldsymbol{k}_\alpha,\alpha} \left( V^1_{\boldsymbol{k}_\alpha} d_1^\dagger c_{\boldsymbol{k}_\alpha} + V^3_{\boldsymbol{k}_\alpha} d_3^\dagger c_{\boldsymbol{k}_\alpha} \right) + H.C \tag{S54}$$

$$= \sum_{\boldsymbol{k}_\alpha,\alpha} \left[ V^1_{\boldsymbol{k}_\alpha} (\varepsilon_1 - \varepsilon_+) + t V^3_{\boldsymbol{k}_\alpha} \right] \frac{\sqrt{(\varepsilon_1 - \varepsilon_-)^2 + t^2}}{(\varepsilon_- - \varepsilon_+)\, t}\, d_-^\dagger c_{\boldsymbol{k}_\alpha}$$

$$- \sum_{\boldsymbol{k}_\alpha,\alpha} \left[ V^1_{\boldsymbol{k}_\alpha} (\varepsilon_1 - \varepsilon_-) + t V^3_{\boldsymbol{k}_\alpha} \right] \frac{\sqrt{(\varepsilon_1 - \varepsilon_+)^2 + t^2}}{(\varepsilon_- - \varepsilon_+)\, t}\, d_+^\dagger c_{\boldsymbol{k}_\alpha} + H.C \tag{S55}$$

$$= \sum_{\boldsymbol{k}_\alpha,\alpha} \left( V^-_{\boldsymbol{k}_\alpha} d_-^\dagger c_{\boldsymbol{k}_\alpha} + V^+_{\boldsymbol{k}_\alpha} d_+^\dagger c_{\boldsymbol{k}_\alpha} \right) + H.C \tag{S56}$$

We note that by tuning the QD parameters such that $\varepsilon_1(R_c, V_{g,c}) - \varepsilon_3(R_c, V_{g,c}) = t\left( \frac{V^1_{\boldsymbol{k}_\alpha}}{V^3_{\boldsymbol{k}_\alpha}} - \frac{V^3_{\boldsymbol{k}_\alpha}}{V^1_{\boldsymbol{k}_\alpha}} \right)$, we obtain $V^1_{\boldsymbol{k}_\alpha} (\varepsilon_1 - \varepsilon_+) + t V^3_{\boldsymbol{k}_\alpha} = 0$, thus decoupling the diagonal level $d_-$. As a consequence, we just see a single peak occurring in the conductance calculation Fig. 3(e) at $(R, V_g) = (R_c, V_{g,c})$.

### C. Estimate for the hopping and broadening terms

We estimate the hybridization parameters through $t_{ij} = \int d\theta dr\, r\, \psi_i^\dagger V_{pert}\, \psi_j$ using $V_{pert} \sim 1$ meV and recalling that $\psi_i = \psi^\sigma_{j_z,n}$, Eq. (6) (main text). Due to time reversal symmetry we have $t_{12} = t_{34} =$

0 for a non-magnetic $V_{pert}$ perturbation. On the other hand, the broadening due to the dot-lead coupling terms are estimated through $\Gamma^{L(R)} = |t|^2 (V_b - \varepsilon_F)$ where $|t|^2 = \left(1 + \frac{V_b^2 \sinh\left[d_b \sqrt{2m_b(V_b - E_f)/\hbar^2}\right]}{4E_f(V_b - E_f)}\right)^{-1}$ is the transmission probability for the electron with energy $\varepsilon_F$ to be transmitted through a barrier with width $d_b = 2.5$nm, height $V_b = 400$meV and effective mass $m_b = 0.14 m_0$ (AlSb mass barrier). Due to the similar wave function profiles of the trivial and topological QD edge states, we have estimated $t_{13} = t_{24} = t = 1$ meV and $\Gamma^{L(R)}_{lm} = 4$ meV for both QDs regimes.

---


[1] P.T. Webster, N.A., Riordan, C. Hogineni, S. Liu, X-H Zhao, D.J. Smith, Y.-H. Zhang, and S.R. Johnson, J. Vac. Soc. & Tech. B **32**, 02C120-1 (2014).

[2] W. H. Lau, J. T. Olesberg and M. E. Flatté, cond-mat/0406201.

[3] B. Andrei Bernevig, Taylor L. Hughes, Shou-Cheng Zhang, Science **314**, 1757, (2006)

[4] P. Michetti, P.H. Penteado, J.C. Egues, and P. Recher, Semicond. Sci. Technol. **27**, 124007 (2012)

[5] J. Shabani, et. al., Phys. Rev. B **93**, 155402, (2016).

[6] R. S. Calsaverini, E. Bernardes, J. C. Egues, and D. Loss, Phys. Rev. B **78**, 155313 (2008).

[7] R. Winkler, *Spin-Orbit Coupling Effects in Two-Dimensional Electron and Hole Systems, Springer Tracts in Modern Physics* Vol. 191 (Springer, New York, 2003).

[8] J. Fu and J. Carlos Egues, Phys. Rev. B **91**, 075408, (2015).

[9] J. Fu et. al., Phys. Rev. Lett. **117**, 226401, (2016)

[10] Rothe D. G., R. W. Reinthaler, C.-X. Liu, L. W. Molenkamp, S. C. Zhang, and E. M. Hankiewicz, New J. Phys., **12**, 065012, (2010).

[11] X.-L. Qi and S. C. Zhang, Rev. Mod. Phys., **83**, 1057, (2011).

[12] J. van Bree, A. Yu. Silov, P. M. Koenraad and M. E. Flatté, Phys. Rev. B. **90**, 165306 (2014)

[13] J. van Bree, A. Yu. Silov, P. M. Koenraad and M. E. Flatté, Phys. Rev. Lett. **112**, 187201 (2014)

[14] Y. Meir, Ned S. Wingreen, Phys. Rev. Lett. **68**, 16 (1992)

[15] M. L. Ladrn de Guevara, et. al., Phys. Rev. B, **67**, 195335 (2003)

[16] G.-H. Ding, et. al., Phys. Rev. B, **71**, 205313 (2005)

[17] H. Lu, et. al., Phys. Rev. B, **71**, 235320 (2005)

[18] J. Antti-Pekka, N. S. Wingreen, and Y. Meir, Phys. Rev. B **50**, 5582 (1994)
